# Supplementary material for: The Gaia Ultracool Dwarf Sample -- IV. GTC/OSIRIS optical spectra of Gaia late-M and L dwarfs
Source: arXiv:2409.03706 source file (2024-09-20)
Supplement: Supplementary file 1 [file obs_dates.tex]

\begin{table}
    \centering
    \begin{tabular}{ccc}
        \hline\textbf{Day} & \textbf{Month} & \textbf{Year} \\ \hline \hline
        31\st & March & 2015 \\ \hline
        1\st & April & 2015\\
        2\nd  & April & 2015 \\
        4\thdate & April & 2015 \\
        5\thdate & April & 2015 \\
        8\thdate & April & 2015 \\
        27\thdate/28\thdate & April & 2015 \\
        29\thdate & April & 2015 \\ \hline
        1\st & May & 2015 \\
        3\rd  & May & 2015 \\
        5\thdate & May & 2015 \\
        28\thdate/ 29\thdate & May & 2015 \\ \hline
        31\st/1\st & June & 2015 \\
        26\thdate & June & 2015 \\ \hline
        7\thdate & July & 2015 \\ \hline
        4\thdate & August & 2015 \\
        6\thdate & August & 2015 \\
        22\nd & August & 2015 \\
        30\thdate & August & 2015 \\
        31\st & August & 2015 \\ \hline
        1\st & September & 2015 \\
        2\nd & September & 2015 \\
        29\thdate & September & 2015 \\ \hline
        1\st & October & 2015 \\ \hline
        28\thdate & November & 2015 \\
        30\thdate & November & 2015 \\ \hline
        30\thdate & December & 2015 \\
        31\st & December & 2015 \\ \hline \hline
        6\thdate & January & 2016 \\ 
        19\thdate & January & 2016 \\
        29\thdate & January & 2016 \\ \hline
        12\thdate & February & 2016 \\
        26\thdate & February & 2016 \\
        27\thdate & February & 2016 \\ \hline
        25\thdate & March & 2016 \\ 
        27\thdate & March & 2016 \\
        28\thdate & March & 2016 \\
        29\thdate & March & 2016 \\ \hline
    \end{tabular}
    \caption{
        Dates of observations, single dates are either early mornings or late evenings,
        a double date for observational blocks that overlay midnight.
    }
\end{table}
