# Supplementary material for: The Gaia Ultracool Dwarf Sample -- IV. GTC/OSIRIS optical spectra of Gaia late-M and L dwarfs
Source: arXiv:2409.03706 source file (2024-09-20)
Supplement: Supplementary file 2 [file spectral_indices.tex]

\onecolumn
\begin{longtable}[c]{l c c cc cc c cc cc}
\caption{ \label{table:spectral-indices}
Spectral indices as defined in \citet{1999ApJ...519..802K, 1999AJ....118.2466M}.}\\
\hline
    Object     &  CrH-a & Colour-d & CrH-1 & CrH-2 & FeH-1 & FeH-2 &
     H$_2$O-1 & VO-1  & VO-2  & Rb-b/TiO-b & Cs-a/VO-b \\
    short name &  Ratio  &  Ratio  & Ratio & Ratio & Ratio & Ratio &
     Ratio  & Ratio & Ratio & Ratio      & Ratio     \\
\hline
\endfirsthead
\hline
    Object     &  CrH-a & Colour-d & CrH-1 & CrH-2 & FeH-1 & FeH-2 &
     H$_2$O-1 & VO-1  & VO-2  & Rb-b/TiO-b & Cs-a/VO-b \\
    short name &  Ratio  &  Ratio  & Ratio & Ratio & Ratio & Ratio &
     Ratio  & Ratio & Ratio & Ratio      & Ratio     \\
\hline
\endhead
\hline
\endfoot
\hline
\endlastfoot
        J0028$-$1927 & 1.3 & 3.4 & 1.3 & 1.7 & 1.4 & 2.2 & 1.1 & 1.1 & 1.1 & 0.9 & 0.4\\
    J0235$-$0849 & 1.5 & 5.8 & 1.4 & 1.9 & 1.5 & 2.3 & 1.2 & 1.0 & 1.2 & 0.9 & 0.5\\
    J0428$-$2253 & 1.3 & 5.5 & 1.2 & 1.7 & 1.3 & 2.0 & 1.2 & 1.1 & 1.2 & 0.9 & 0.5\\
    J0453$-$1751 & 1.5 & 5.4 & 1.4 & 1.9 & 1.5 & 2.2 & 1.2 & 1.0 & 1.1 & 1.3 & 0.5\\
    J0502$+$1442 & 1.1 & 4.2 & 1.0 & 1.5 & 1.0 & 1.8 & 1.2 & 1.4 & 1.2 & 0.6 & 0.4\\
    J0605$-$2342 & 1.2 & 5.3 & 1.2 & 1.7 & 1.2 & 2.1 & 1.2 & 1.2 & 1.2 & 0.8 & 0.4\\
    J0741$+$2316 & 1.1 & 3.5 & 1.1 & 1.3 & 1.0 & 1.6 & 1.3 & 1.2 & 1.1 & 0.7 & 0.4\\
    J0752$+$4136 & 1.0 & 1.8 & 1.0 & 1.2 & 1.0 & 1.5 & 1.2 & 1.2 & 1.3 & 0.8 & 0.5\\
    J0809$+$2315 & 2.1 & 7.9 & 1.8 & 1.6 & 1.6 & 2.1 & 1.3 & 0.7 & 1.1 & 1.9 & 0.5\\
    J0823$+$0240 & 1.1 & 3.5 & 1.0 & 1.4 & 1.1 & 1.8 & 1.3 & 1.3 & 1.3 & 0.6 & 0.4\\
    J0823$+$6125 & 1.5 & 4.2 & 1.4 & 1.6 & 1.5 & 1.9 & 1.1 & 1.0 & 1.1 & 1.2 & 0.5\\
    J0829$-$1309 & 1.3 & \ldots & 1.3 & \ldots & 1.2 & \ldots & \ldots & 1.0 & 1.2 & 0.9 & 0.4\\
    J0847$-$1532 & 1.2 & \ldots & 1.3 & \ldots & 1.4 & \ldots & \ldots & 0.9 & 1.2 & 0.8 & 0.4\\
    J0918$+$2134 & 1.5 & 4.7 & 1.4 & 1.6 & 1.5 & 1.8 & 1.0 & 0.9 & 1.1 & 1.4 & 0.6\\
    J0935$-$2934 & 1.2 & 4.5 & 1.2 & 1.6 & 1.2 & 2.0 & 1.2 & 1.2 & 1.3 & 0.8 & 0.4\\
    J0938$+$0443 & 1.0 & 3.3 & 1.0 & 1.3 & 1.0 & 1.5 & 1.2 & 1.4 & 1.2 & 0.6 & 0.4\\
    J0940$+$2946 & 1.5 & 5.5 & 1.4 & 1.8 & 1.5 & 2.2 & 1.1 & 1.0 & 1.2 & 1.0 & 0.5\\
    J0953$-$1014 & 1.0 & 5.4 & 1.0 & 1.3 & 0.9 & 1.5 & 1.2 & 1.5 & 1.1 & 0.6 & 0.3\\
    J1004$+$5022 & 1.3 & 4.4 & 1.3 & 1.4 & 1.4 & 1.5 & 1.1 & 0.8 & 1.1 & 1.1 & 0.5\\
    J1004$-$1318 & 1.7 & 6.0 & 1.6 & 1.9 & 1.6 & 2.4 & 1.2 & 0.9 & 1.2 & 1.2 & 0.6\\
    J1045$-$0149 & 1.0 & \ldots & 1.1 & \ldots & 0.9 & \ldots & \ldots & 1.0 & 1.3 & 1.0 & 0.6\\
    J1047$-$1815 & 1.4 & 5.0 & 1.3 & 1.9 & 1.5 & 2.3 & 1.1 & 0.8 & 1.2 & 0.9 & 0.5\\
    J1057$+$0623 & 1.0 & 2.7 & 1.1 & 0.5 & 1.0 & 0.7 & 1.3 & \ldots & 1.0 & 1.0 & 0.4\\
    J1058$-$1548 & 1.8 & 5.9 & 1.7 & 1.9 & 1.6 & 2.3 & 1.0 & 0.7 & 1.2 & 1.2 & 0.6\\
    J1109$-$1606 & 1.2 & 3.4 & 1.2 & 1.7 & 1.3 & 2.2 & 1.3 & 1.1 & 1.2 & 0.8 & 0.4\\
    J1127$+$4705 & 1.5 & 3.8 & 1.4 & 2.0 & 1.5 & 2.6 & 1.1 & 0.8 & 1.3 & 0.8 & 0.4\\
    J1213$-$0432 & 2.1 & 10.1 & 1.9 & 1.9 & 1.8 & 2.1 & 1.0 & 0.5 & 1.4 & 1.6 & 0.8\\
    J1216$+$4927 & 1.6 & 5.0 & 1.5 & 1.7 & 1.6 & 2.2 & 1.1 & 1.0 & 1.2 & 1.1 & 0.5\\
    J1221$+$0257 & 1.2 & 4.7 & 1.1 & 1.6 & 1.2 & 2.1 & 1.1 & 1.3 & 1.2 & 0.7 & 0.4\\
    J1222$+$1407 & 1.1 & \ldots & 1.0 & \ldots & 1.0 & \ldots & \ldots & 1.2 & 1.0 & 0.9 & 0.3\\
    J1232$-$0951 & 1.3 & 6.0 & 1.2 & 1.6 & 1.2 & 2.2 & 1.1 & 1.2 & 1.3 & 0.7 & 0.4\\
    J1246$+$4027 & 1.8 & 7.4 & 1.7 & 1.8 & 1.7 & 2.1 & 1.2 & 0.7 & 1.3 & 1.4 & 0.7\\
    J1315$+$1126 & 1.0 & 3.3 & 1.0 & 1.2 & 1.1 & 1.3 & 1.2 & \ldots & 1.0 & 1.0 & 0.4\\
    J1331$+$3407 & 1.2 & 4.6 & 1.2 & 1.6 & 1.2 & 1.9 & 1.1 & 1.0 & 1.1 & 0.8 & 0.4\\
    J1333$-$0215 & 1.5 & 4.6 & 1.4 & 1.7 & 1.5 & 2.2 & 1.1 & 1.0 & 1.1 & 1.1 & 0.5\\
    J1337$+$4938 & 0.8 & \ldots & 0.8 & \ldots & 0.6 & \ldots & \ldots & 0.3 & 1.6 & 1.2 & 0.7\\
    J1346$+$0842 & 1.5 & 4.7 & 1.4 & 1.8 & 1.5 & 2.2 & 1.1 & 1.0 & 1.2 & 1.1 & 0.5\\
    J1412$+$1633 & 1.3 & 4.5 & 1.2 & 1.6 & 1.2 & 2.0 & 1.0 & 1.2 & 1.2 & 0.9 & 0.4\\
    J1421$+$1827 & 1.1 & 4.3 & 1.0 & 1.3 & 1.0 & 1.6 & 1.1 & 1.4 & 1.1 & 0.7 & 0.4\\
    J1439$+$0039 & 1.0 & \ldots & 0.9 & \ldots & 1.2 & \ldots & \ldots & 1.4 & 1.0 & 0.8 & 0.4\\
    J1441$-$0945 & 1.3 & 5.3 & 1.2 & 1.5 & 1.3 & 1.8 & 1.4 & 1.1 & 1.2 & 0.9 & 0.4\\
    J1506$+$1321 & 1.1 & \ldots & 1.2 & \ldots & 1.9 & \ldots & \ldots & 0.3 & 1.2 & 2.0 & 0.3\\
    J1526$+$2808 & 1.3 & 1.9 & 1.2 & 1.6 & 1.3 & 2.0 & 0.9 & 1.0 & 1.0 & 0.9 & 0.5\\
    J1527$+$0553 & 0.9 & \ldots & 1.0 & \ldots & 1.0 & \ldots & \ldots & 1.3 & 1.1 & 0.7 & 0.4\\
    J1532$+$2611 & 1.6 & 6.1 & 1.6 & 1.9 & 1.6 & 2.4 & 1.0 & 0.9 & 1.2 & 1.1 & 0.5\\
    J1539$-$0520 & 1.7 & 38.8 & 1.6 & 2.2 & 1.7 & 2.8 & 1.2 & 0.8 & 1.3 & 1.2 & 0.6\\
    J1548$-$1636 & 1.1 & 4.4 & 1.0 & 1.4 & 1.0 & 1.7 & 1.2 & 1.4 & 1.2 & 0.6 & 0.4\\
    J1617$+$7733B & 1.0 & 1.6 & 0.9 & 1.1 & 0.9 & 1.3 & 1.2 & 1.2 & 1.3 & 0.8 & 0.5\\
    J1618$-$1321 & 1.2 & 4.5 & 1.1 & 1.5 & 1.2 & 1.9 & 1.0 & 1.0 & 1.1 & 0.7 & 0.4\\
    J1623$+$1530 & 1.1 & 5.3 & 1.1 & 1.5 & 1.1 & 1.9 & 1.3 & 1.3 & 1.3 & 0.6 & 0.4\\
    J1623$+$2908 & 1.2 & 12.3 & 1.2 & 1.5 & 1.4 & 2.1 & 1.0 & 1.0 & 1.2 & 0.9 & 0.5\\
    J1705$-$0516 & 1.3 & \ldots & 1.2 & \ldots & 1.3 & \ldots & \ldots & 1.1 & 1.2 & 0.8 & 0.4\\
    J1707$-$0138 & 1.5 & 7.3 & 1.4 & 1.8 & 1.5 & 2.5 & 1.3 & 1.0 & 1.3 & 0.9 & 0.5\\
    J1717$+$6526 & 1.7 & 14.0 & 1.6 & 1.4 & 1.4 & 1.5 & 1.1 & 0.6 & 1.6 & 1.9 & 0.7\\
    J1724$+$2336 & 1.0 & \ldots & 1.0 & \ldots & 1.0 & \ldots & \ldots & 1.3 & 1.3 & 0.7 & 0.4\\
    J1733$-$1654 & 1.4 & 1.0 & 1.3 & 1.0 & 1.5 & 1.0 & 1.2 & 0.9 & 1.3 & 0.8 & 0.4\\
    J1745$-$1640 & 1.4 & 5.1 & 1.3 & 1.6 & 1.4 & 2.2 & 1.4 & 1.1 & 1.1 & 0.9 & 0.4\\
    J1750$-$0016 & 1.9 & 9.3 & 1.8 & 1.7 & 1.6 & 1.9 & 1.0 & 0.5 & 1.4 & 1.9 & 0.8\\
    J2155$+$2345 & 1.8 & 3.7 & 1.6 & 1.9 & 1.7 & 2.2 & 1.0 & 0.8 & 1.2 & 1.2 & 0.6\\
    J2339$+$3507 & 1.9 & 5.4 & 1.8 & 1.7 & 1.7 & 2.1 & 1.0 & 0.8 & 1.2 & 1.2 & 0.6\\

\end{longtable}
\clearpage
\twocolumn
